# Supplementary material for: Scaling Deep Learning Computation over the Inter-Core Connected Intelligence Processor with T10
Source: arXiv:2408.04808 source file (2024-09-24)
Supplement: Supplementary file 1 [file appendix.tex]

\appendix

\section{Constraints on Rotating Pace in \S\ref{sec:design:compute}}
\label{appendix:rp_constraint}

In \S\ref{sec:design:compute}, we define the constraints on rotating paces in \Cref{eqn:rp_constraint}.
\rtensor{}s $\{1,2,\dots,i\}$ rotating along axis $k$ must share the same $\rp$ value on $k$. Also, the shared $\rp$ value on $k$ has:
$$rp \leq \frac{K}{2f_t^{i}}+\frac{1}{2} \textbf{ } \textbf{ or } \textbf{ } rp=\frac{K}{f_{t}^{i}}\text{ ,}$$
where $f_t^i$ is temporal partition factor of \rtensor{} $i$ along $k$, and $K$ is the length of dimension $k$ in number of elements.

The compute-shift paradigm assumes the following conditions:
First, for each step, each sub-operator computes a sub-task whose shape aligns with the rotating pace along each rotated dimension.
For example, if $\rp=3$ on $k$, then the sub-task must have a shape $[\dots,3,\dots]$ for axes $[\dots,k,\dots]$.
Second, sub-tasks on cores of a same rotating ring 

Each sub-operator iterates over all its sub-tasks by nested-looping through the axes of this operator.
Between sub-tasks, an \rtensor{} is rotated along the currently iterating axis for all its sub-tensors. The process continues until all sub-tasks are enumerated.

% The intuition is that if the original $K/f_t^i$-sized partitions of some \rtensor{}s are unaligned (i.e., there exist two \rtensor{}s $i$ and $j$ such that $K/f_t^i \neq K/f_t^j$), we want to find an appropriate $\rp$ to reorganize each \rtensor{} into $\rp$-sized partitions and maintain the data dependency.

% $$rp \leq \frac{K}{2f_t^{i}}+\frac{1}{2} \textbf{ } \textbf{ or } \textbf{ } rp=\frac{K}{f_{t}^{i}}$$
\begin{figure}[!tph]
    \centering
    % \vspace{-1ex}
    \includegraphics[scale=0.88]{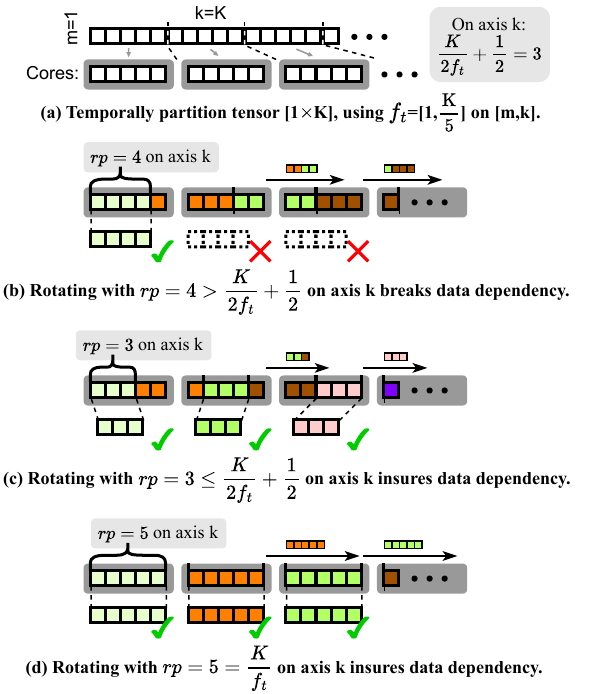}
    \vspace{-5ex}
    \caption{Constrains on the values of rotating pace.}
    \label{fig:rp_constraint}
    \vspace{-1ex} 
\end{figure}
